# Supplementary material for: Differentiable Retrieval Augmentation via Generative Language Modeling for E-commerce Query Intent Classification
Source: arXiv:2308.09308 source file (2023-09-15)
Supplement: Supplementary file 1 [file 6-appendix.tex]

\section{Appendix}
